# Supplementary material for: Efficient and rate-optimal list-decoding in the presence of minimal feedback
Source: arXiv:2511.04088 source file (2026-11-17)
Supplement: Supplementary file 1 [file q-ary-entrop-approx.tex]

\section{Approximation to the $q$-ary entropy function} \label{sec:q-ary_approx}

The capacity of a $q$-ary symmetric channel (in bits) equals

\begin{align}
\log_2(q) - p\log_2(q-1) - H_2(p) & =  p\log_2\left ( \frac{q}{q-1}\right ) + (1-p)\log_2(q) +p\log_2(p) + (1-p)\log_2(1-p) \\
& =  p\log_2\left ( \frac{p}{1-1/q}\right ) + \left ( \frac{1-p}{1/q}\right ) \\
& =  D(p||1-1/q)
\end{align}

Say $p<1-1/q -  \gamma$. By Pinsker's inequality,  $$D(p||1-1/q) \geq\frac{\gamma^2}{2\ln2}$$
